# Supplementary material for: Membership Inference Attack Using Self Influence Functions
Source: arXiv:2205.13680 source file (2022-05-26)
Supplement: Supplementary file 1 [file intro.tex]

The supplementary material is organized as follows:
\begin{itemize}
    
\item Appendix~\ref{supp_sec:sif_algorithm} provides pseudo codes to outline the fitting and inference of our membership inference (MI) attack model.

\item Appendix~\ref{supp_sec:efficient_sif_calculation} explains in detail how the self-influence measure was approximated for SIF and adaSIF.

\item Appendix~\ref{supp_sec:hardware_setup} lists the hardware (CPUs \& GPUs) we used for training the target models and for fitting/evaluating our attack models.

\item Appendix~\ref{supp_sec:accuracy_of_target_models} reports the train/test accuracies for all the target models.

\item Appendix~\ref{supp_sec:comparison_of_mi_attacks} compares our MI attack to baselines for target models trained on AlexNet and DenseNet architectures.

\item Appendix~\ref{supp_sec:precision_and_recall} reports the precision and recall metrics on members and non-members, for our attack model and baselines.

\item Appendix~\ref{supp_sec:naive_sif_ensemble} advocates the use of our proposed adaSIF over a naive SIF ensemble.

\item Appendix~\ref{supp_sec:comparison_of_mi_attacks_with_data_augmentation} compares the attack performance of adaSIF to baselines, for target models trained with data augmentations on AlexNet and DenseNet.

\item Appendix~\ref{supp_sec:comparison_to_a_white_box_attack} compares our MI attack methods to an additional white-box attack.

\end{itemize}
