# Supplementary material for: Membership Inference Attack Using Self Influence Functions
Source: arXiv:2205.13680 source file (2022-05-26)
Supplement: Supplementary file 2 [file 0_metadata.tex]

\title{Membership Inference Attack Using\\ Self Influence Functions\\ (Supplementary Material)}

% The \author macro works with any number of authors. There are two commands
% used to separate the names and addresses of multiple authors: \And and \AND.
%
% Using \And between authors leaves it to LaTeX to determine where to break the
% lines. Using \AND forces a line break at that point. So, if LaTeX puts 3 of 4
% authors names on the first line, and the last on the second line, try using
% \AND instead of \And before the third author name.

\author{%
  Anonymous Author(s) \\
}
